# Supplementary material for: Universal Nucleation Behaviour of Sheared Systems
Source: arXiv:2011.01020 source file (2021-01-07)
Supplement: Supplementary file 1 [file supplementary.pdf]

# Supporting Information: Universal Nucleation Behavior of Sheared Systems

Amrita Goswami, Indranil Saha Dalal,* and Jayant K. Singh*

*Department of Chemical Engineering, Indian Institute of Technology Kanpur*

E-mail: indrasd@iitk.ac.in; jayantks@iitk.ac.in

## 1 Simulation Details

Equilibrium and non-equilibrium molecular dynamics (NEMD) trajectories were obtained using LAMMPS (Large-scale Atomic/Molecular Massively Parallel Simulator).[S1] The SLLOD algorithm[S2] and the Lees-Edwards boundary conditions[S3,S4] were used to generate simple shear flows in the $x$ dimension. The Nose-Hoover thermostat was used to control the temperature.[S5]

We have analyzed five different systems in this work: the rigid water models TIP4P/2005[S6] and TIP4P/Ice,[S7] the coarse-grained monoatomic water (mW) model,[S8] the truncated and shifted Lennard-Jones (LJ) potential[S9] for Argon, and a hard-sphere (HS) colloid.

We simulated the mW model at 235 $K$, 240 $K$, 255 $K$, and 260 $K$. We used a time-step of 5 $fs$ for the Velocity-Verlet integration scheme. The system size was 4096 water molecules.

Temperatures of 237.5 $K$, 232.5 $K$ and 232.5 $K$ were simulated for the TIP4P/2005 model, corresponding to supercoolings of 14.5 $K$, 19.5 $K$ and 29.5 $K$, respectively. For TIP4P/Ice, simulations were performed for supercoolings of 14.5 $K$, 19.5 $K$ and 34.5 $K$, at

temperatures of 257.5 $K$, 252.5 $K$, and 237.5 $K$, respectively. The long-range electrostatics were treated with the particle-particle particle-mesh (PPPM) algorithm.[S10] The rigid water molecules were constrained by the SHAKE algorithm.[S11] Systems were composed of 4029 water molecules for both TIP4P/2005 and TIP4P/Ice.

Reduced units, in terms of the depth of the interaction potential, $\epsilon$, and the distance at which the potential vanishes, $\sigma$, have been used throughout for the LJ potential. The LJ interactions were truncated at 8.5 Å. The number of atoms in the simulations was 13500, and the density at each temperature was taken to be that at a pressure of $-0.02\epsilon/\sigma^3$.

For TIP4P/2005, TIP4P/Ice, mW and LJ, the two-dimensional diffusion coefficients in the absence and presence of shear were calculated using the VMD Diffusion Coefficient Tool.[S12] Long simulation times of at least 200 $ns$ for mW and LJ, and $\approx 100-200$ $ns$ for the rigid water models were maintained to ensure that the linear diffusive regime was attained.

The viscosity at each temperature for every model was estimated by a nonequilibrium method with periodic shear flow.[S13] Errors were estimated from $6-8$ independent NEMD simulations for each data point.

# 2 Supplementary Tables and Figures

Table S1: Shear viscosities at various temperatures and 1 *atm* for the water models studied in this work.

| Model | Temperature (K) | Viscosity (mPas) | Experiment (mPas) |
|---|---|---|---|
| TIP4P/2005 | 237.5 | $12.44 \pm 0.98$ | $15.3 \pm 3$[S14] |
| TIP4P/2005 | 232.5 | $24.79 \pm 1.08$ | - |
| TIP4P/2005 | 222.5 | $117.6 \pm 12.2$ | - |
| TIP4P/Ice | 257.5 | $15.4 \pm 0.29$ | $3.558 \pm 0.156$[S15] |
| TIP4P/Ice | 252.5 | $23.17 \pm 0.76$ | $4.738 \pm 0.21$[S15] |
| TIP4P/Ice | 237.5 | $175.3 \pm 10$ | $15.3 \pm 3$[S14] |
| mW | 260 | $0.487 \pm 0.0057$ | $3.059 \pm 0.134$[S15] |
| mW | 255 | $0.519 \pm 0.0062$ | $3.967 \pm 0.174$[S15] |
| mW | 240 | $0.683 \pm 0.006$ | $12.68 \pm 0.555$[S15] |
| mW | 235 | $0.683 \pm 0.006$ | $25.88 \pm 1.13$[S15] |

Table S2: Values of $D_0$ and $c$ for the TIP4P/2005, TIP4P/Ice and mW models. The data for the mW model were obtained from Goswami et al.[S16].

| Model | Temperature (K) | $D_0$ ($\times 10^{-11}$ $m^2/s$) | $c$ ($\times 10^{-20}$ $m^2$) |
|---|---|---|---|
| TIP4P/2005 | 237.5 | 15.08 | 1.18 |
| TIP4P/2005 | 232.5 | 7.73 | 1.25 |
| TIP4P/2005 | 222.5 | 2.92 | 1.20 |
| TIP4P/Ice | 257.5 | 15.16 | 1.19 |
| TIP4P/Ice | 252.5 | 9.47 | $1.17 |
| TIP4P/Ice | 237.5 | 1.72 | 1.22 |
| mW | 260 | 371.5 | 0.485 |
| mW | 255 | 334.5 | 0.533 |
| mW | 240 | 249.6 | 0.617 |
| mW | 235 | 214.5 | 0.663 |

Table S3: Values of the interfacial energy $\sigma_0$, chemical potential $|\Delta\mu_0|$, volume of a single ice molecule $v'$, liquid density $\rho_l$, required for the calculation of the nucleation rate for the water models studied in this work. The attachment length $\lambda$ has been taken to be 3.5 Å for all cases. $\sigma_0$ and $|\Delta\mu_0|$ were obtained from Espinosa et al.[S17].

| Model | Temperature (K) | $\sigma_0$ (mN/m) | $|\Delta\mu_0|$ (kcal/mol) | $v'$ ($10^{-29}$ $m^3$) | $\rho_l$ ($g/cm^3$) |
|---|---|---|---|---|---|
| TIP4P/2005 | 237.5 | 25.9 | 0.0612 | 3.242 | 0.970 |
| TIP4P/2005 | 232.5 | 25.0 | 0.0801 | 3.238 | 0.967 |
| TIP4P/2005 | 222.5 | 20.4 | 0.1137 | 3.235 | 0.925 |
| TIP4P/Ice | 257.5 | 26.3 | 0.0629 | 3.555 | 0.952 |
| TIP4P/Ice | 252.5 | 25.4 | 0.0826 | 3.292 | 0.947 |
| TIP4P/Ice | 237.5 | 23.7 | 0.1335 | 3.285 | 0.932 |
| mW | 260 | 29.5 | 0.0669 | 3.0534 | 1.0022 |
| mW | 255 | 29.0 | 0.0895 | 3.0503 | 1.0024 |
| mW | 240 | 28.9 | 0.1553 | 3.0441 | 1.0031 |
| mW | 235 | 28.55 | 0.1746 | 3.044 | 1.0031 |

Table S4: Shear viscosities at various temperatures, for the Lennard-Jones system.

| Temperature ($\epsilon/k_B$) | $\eta^*$ ($\epsilon\tau/\sigma^3$) |
|---|---|
| 0.587 | $3.825 \pm 0.012$ |
| 0.572 | $4.176 \pm 0.011$ |
| 0.534 | $5.145 \pm 0.015$ |

Table S5: Values of $D_0$ and $c$ for the Lennard-Jones system.

| Temperature ($\epsilon/k_B$) | $D_0$ ($\sigma^2/\tau$) | $c$ ($\sigma^2$) |
|---|---|---|
| 0.587 | 0.0831 | 0.2014 |
| 0.572 | 0.0748 | 0.1608 |
| 0.534 | 0.0549 | 0.1458 |

Table S6: Values of parameters required for the calculation of the nucleation rate for the LJ system. $\sigma_0$, $|\Delta\mu_0|$, $v'$ and $\lambda$ were obtained from Espinosa et. al.[S18] The shear modulus $G$ used was $23.8\epsilon/\sigma^3$.[S19,S20]

| Temperature ($\epsilon/k_B$) | $\sigma_0$ ($\epsilon/\sigma^2$) | $|\Delta\mu_0|$ ($k_BT$) | $v'$ ($\sigma^3$) | $\lambda$ ($\sigma$) | $\rho_l$ ($\sigma^{-3}$) |
|---|---|---|---|---|---|
| 0.587 | 0.348 | 0.084 | 2.31 | 1 | 0.843 |
| 0.572 | 0.342 | 0.127 | 2.35 | 0.73 | 0.851 |
| 0.534 | 0.33 | 0.246 | 2.69 | 1.15 | 0.868 |

Table S7: Values of input parameters required for the calculation of the nucleation rate for hard spheres (HS). $G$, $\sigma_0$, $|\Delta\mu_0|$ were obtained from Gasser et. al.,[S21] for a HS colloidal suspension of poly(methylmethacrylate) (PMMA) spheres in a mixture of decahydronaphthalene and cyclohexylbromide. The radius of the particles was taken to be $1.26\mu m$. The viscosity $\eta$ was estimated by Mura et. al.[S22] for this system. $D_0$ and $c$ were estimated from the modified Stokes-Einstein relation $D_0 = (\rho_l)^{\frac{1}{3}} \frac{k_B T}{6\eta}$[S23] and Eq.(6), respectively.

| $\phi$ | $D_0$ ($m^2/s$) | $c$ ($m^2$) | $\eta$ (Pa s) | $G$ (Pa) | $\sigma_0$ (N/m) | $\|\Delta\mu_0\|$ (J) |
|---|---|---|---|---|---|---|
| 0.503 | $9.36 \times 10^{-16}$ | $1.28 \times 10^{-12}$ | 0.18 | 0.0016 | $6.87 \times 10^{-11}$ | $5.25 \times 10^{-22}$ |

Table S8: The melting temperatures, $T_m$ for the water models and LJ system used in this work.

| Model | $T_m$ (K) |
|---|---|
| TIP4P/2005 | 252[S6] |
| TIP4P/Ice | 272[S24] |
| mW | 274.6[S8] |
| LJ | 74[S25] |

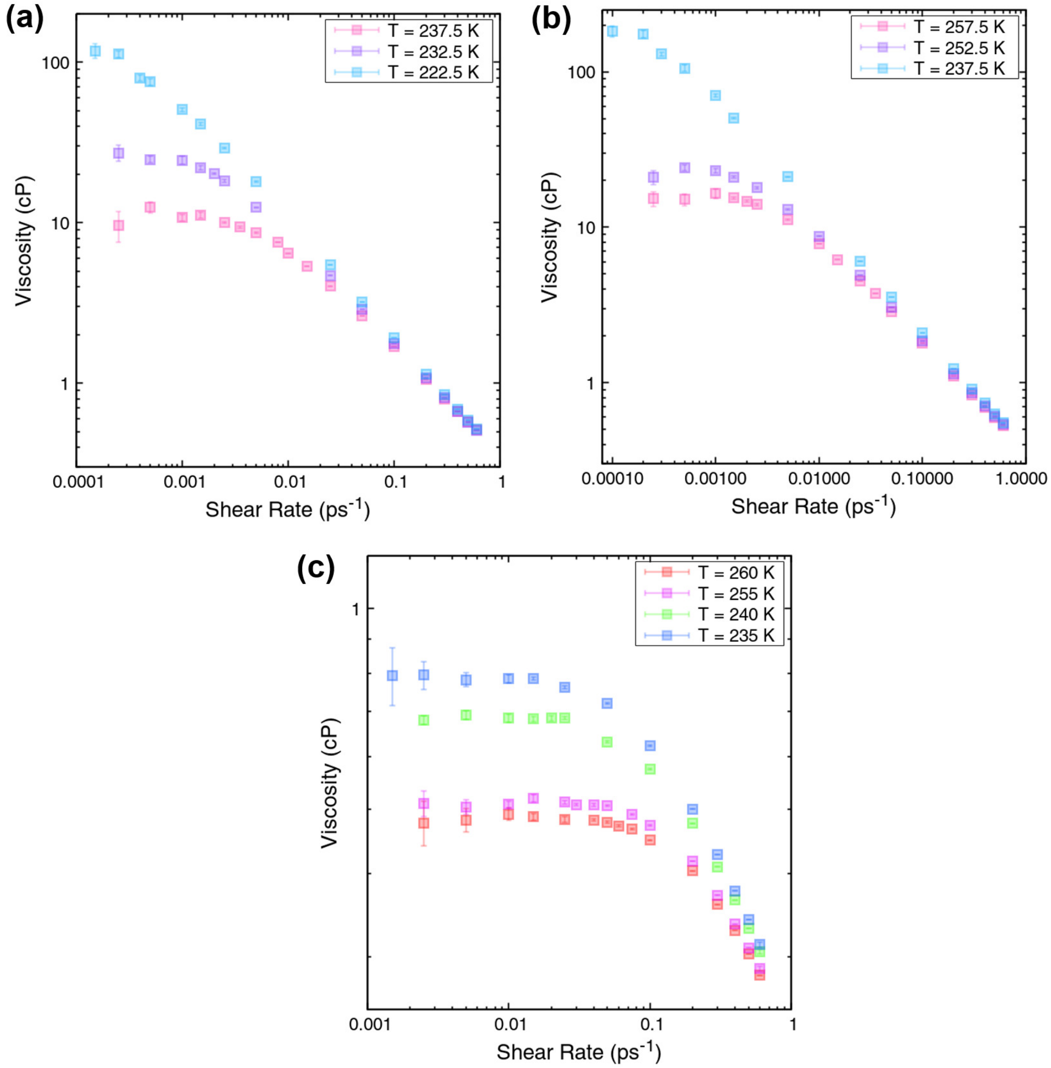


Figure S1: Shear viscosities obtained from NEMD simulations, for the (a) TIP4P/2005 model, (b) TIP4P/Ice model, and (c) mW model. Each transclucent square symbol represents the viscosity for a particular shear rate and temperature, color-coded according to the legend.

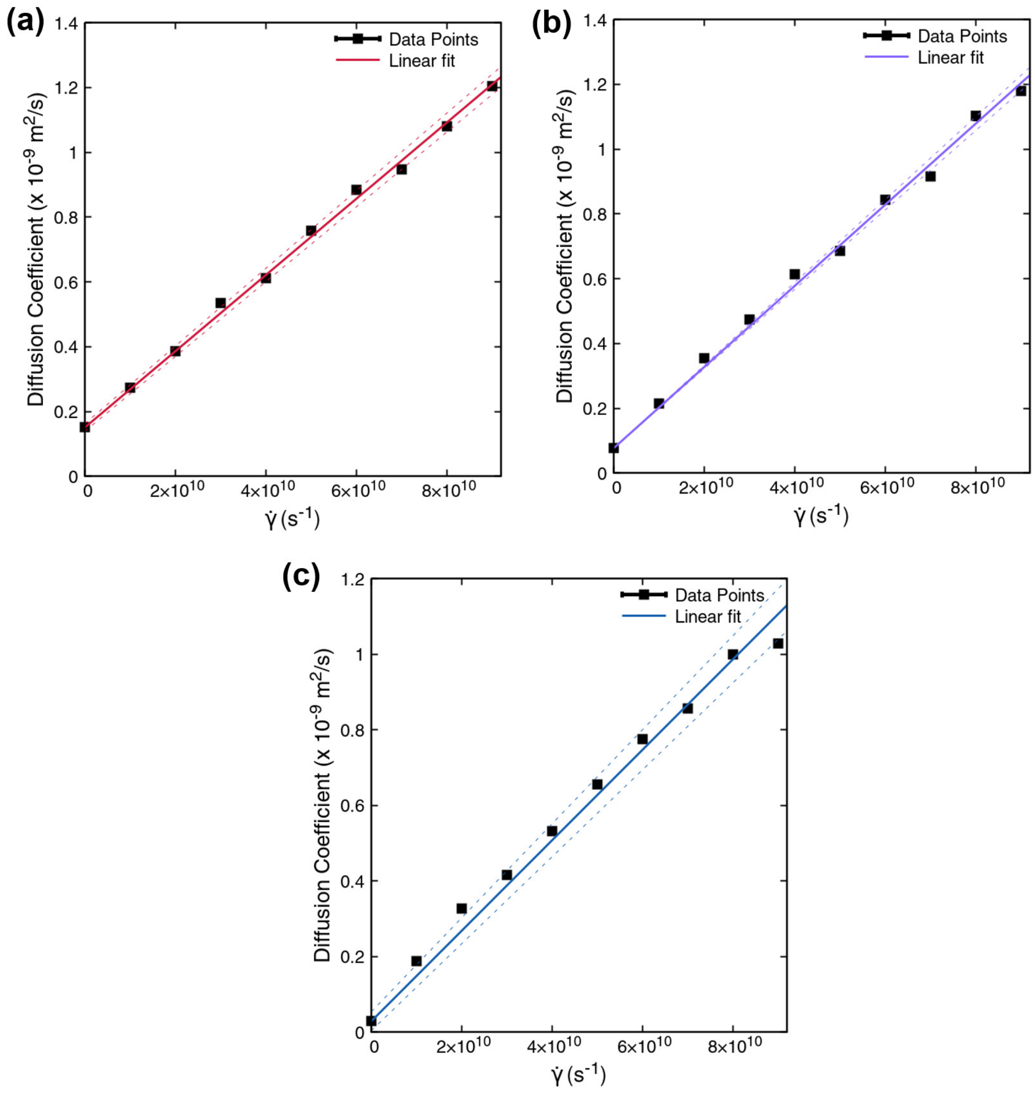


Figure S2: Linear fits of the diffusion coeffcient, $D_l$, at different shear rates, for the TIP4P/2005 model at (a) 237.5 $K$, (b) 232.5 $K$, and (c) 222.5 $K$.

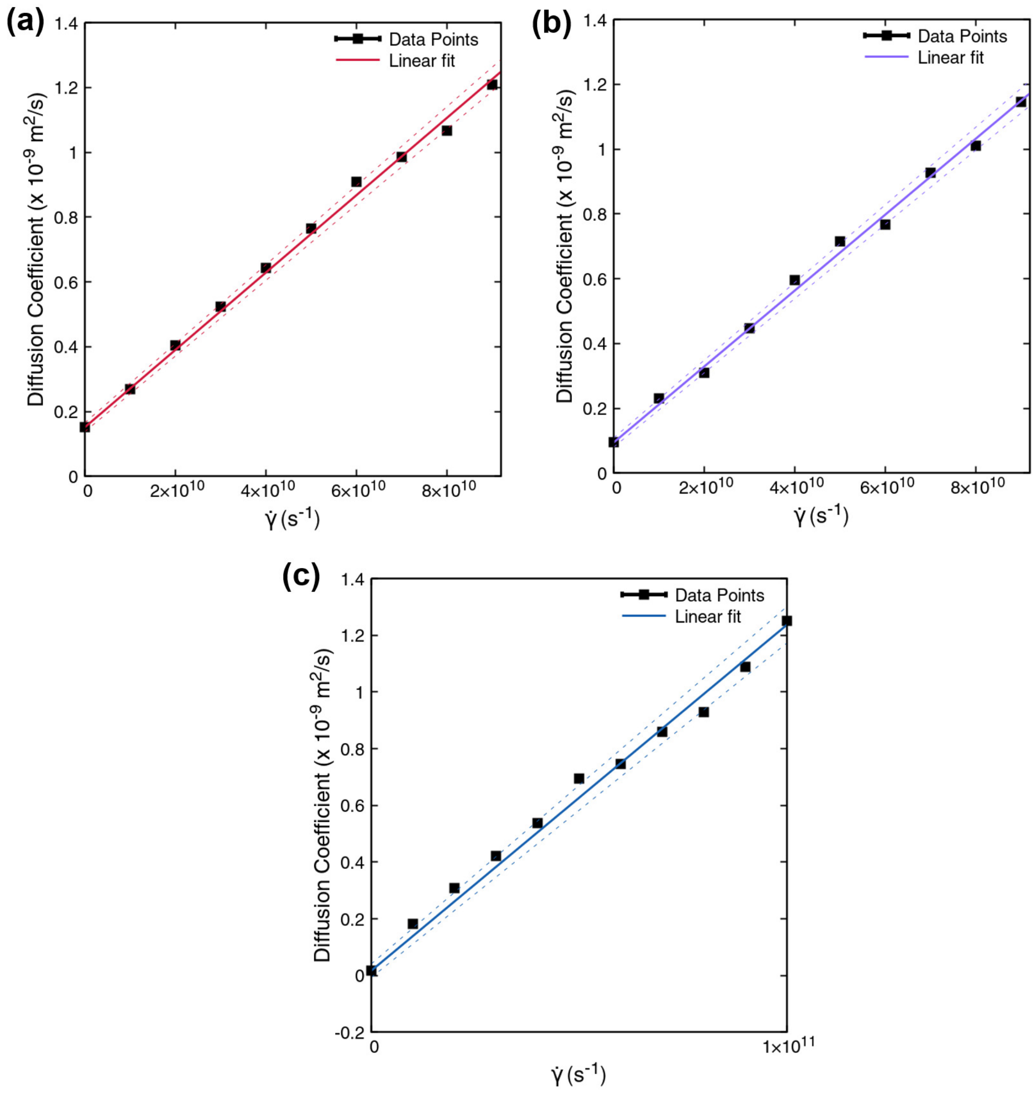


Figure S3: Linear fits of the diffusion coeffcient, $D_l$, at different shear rates, for the TIP4P/Ice model at (a) 257.5 $K$, (b) 252.5 $K$, and (c) 237.5 $K$.

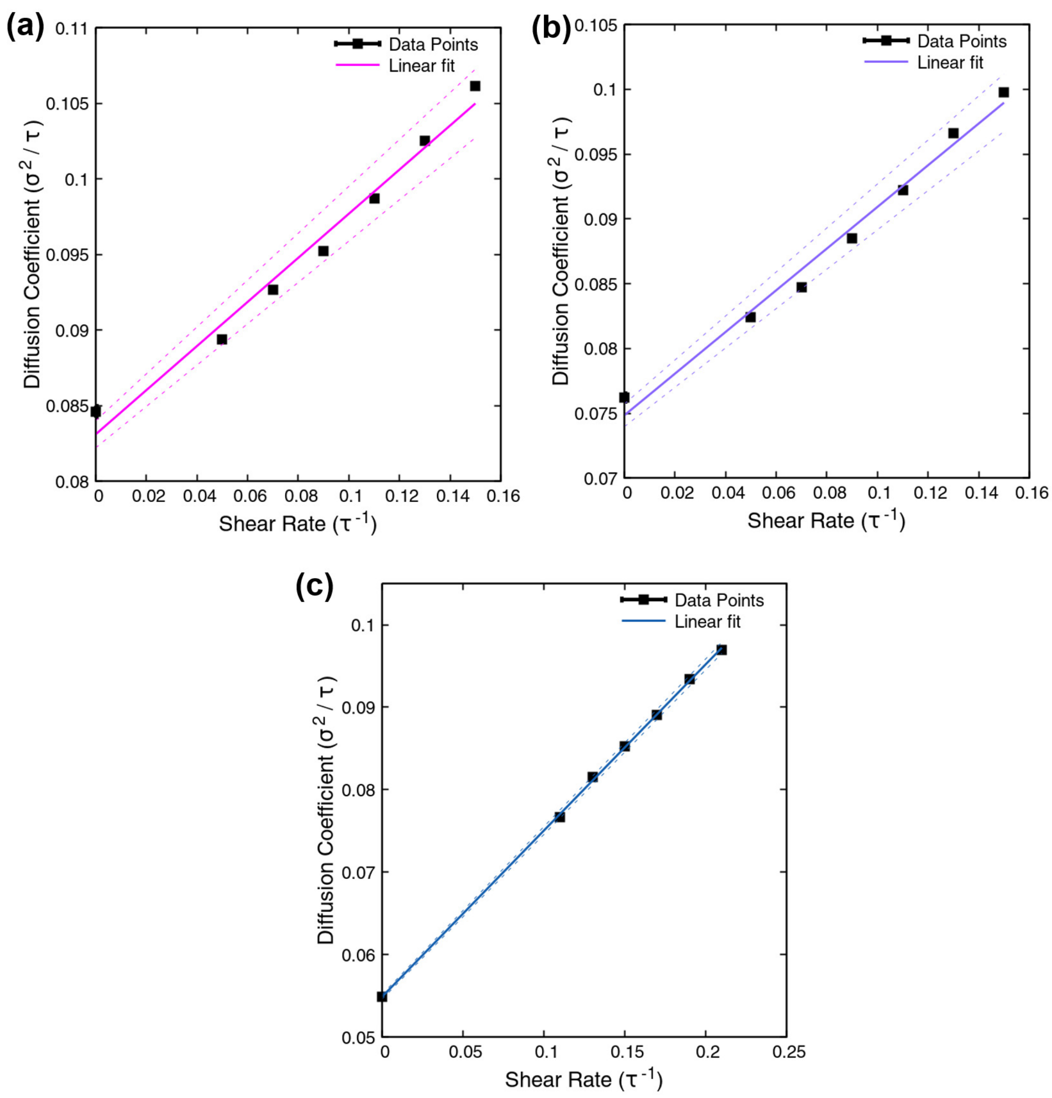


Figure S4: Linear fits of the diffusion coeffcient, $D_l$, at different shear rates, for the LJ system for reduced temperatures of (a) 0.587 $K$, (b) 0.572 $K$, and (c) 0.534 $K$.

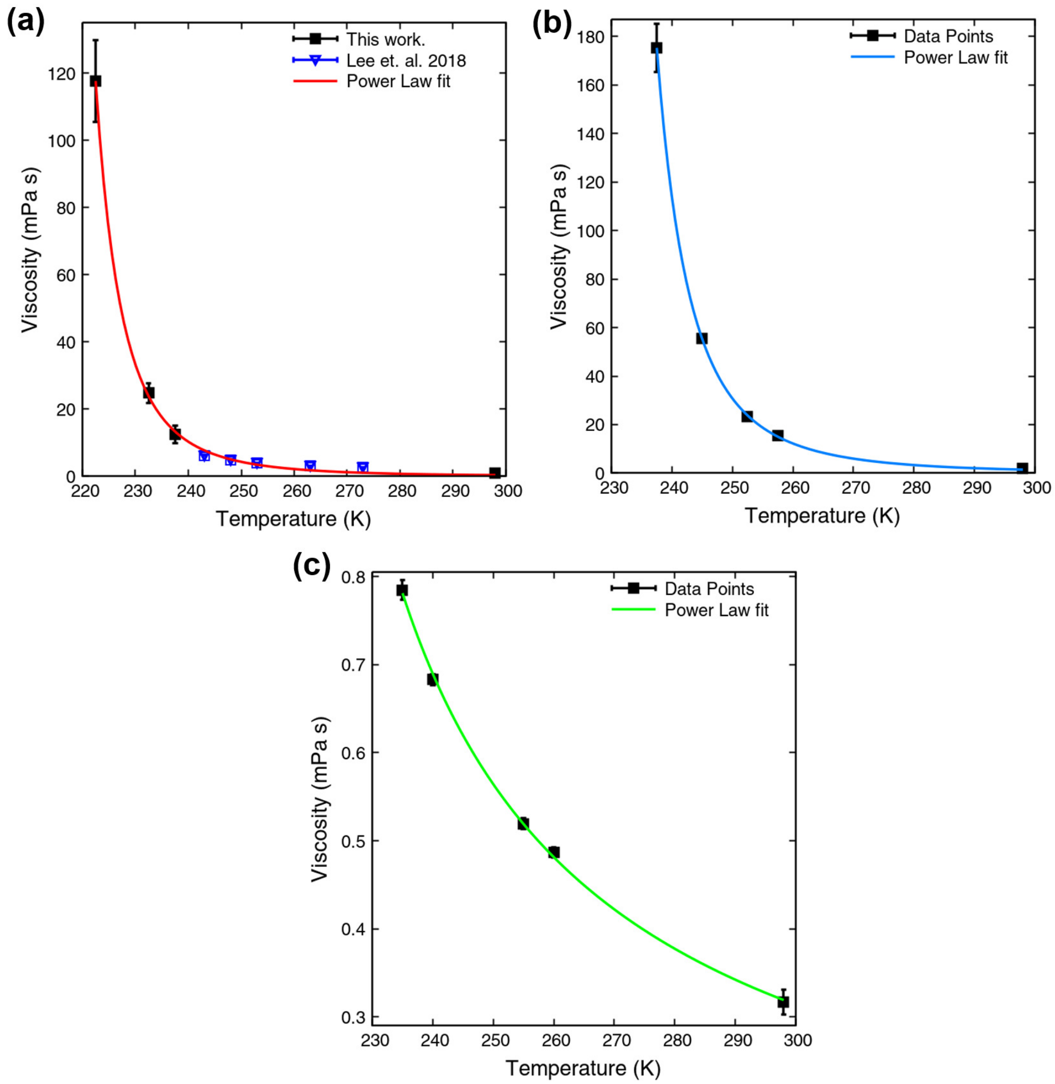


Figure S5: Power law fits to the shear viscosities for the (a) TIP4P/2005 model, (b) TIP4P/Ice model, and (c) mW model. The fitted expression $A_0(\frac{T}{T_s} - 1)^{-\gamma}$ has been shown by solid lines in red, blue and green for the TIP4P/2005, TIP4P/Ice and mW water models. The black filled square symbols denote the viscosity values obtained from NEMD simulations. The filled blue triangles show the shear viscosities calculated by Lee and Kim[S26], for the TIP4P/2005 model.

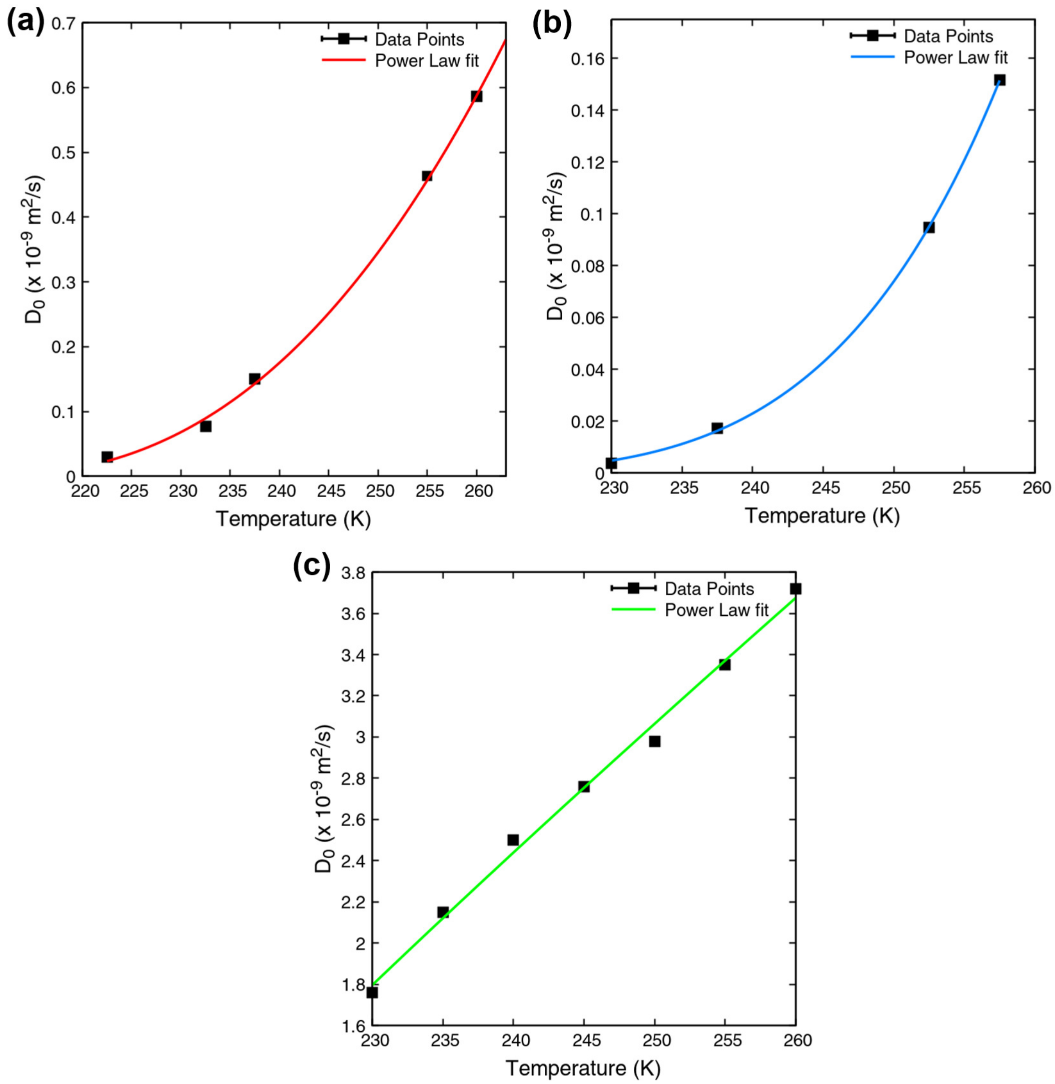


Figure S6: Power law fits to the diffusion coefficients at zero shear, $D_0$, for the (a) TIP4P/2005 model, (b) TIP4P/Ice model, and (c) mW model. Solid lines in red, blue and green depict the fitted power law expression for the TIP4P/2005, TIP4P/Ice and mW water models, respectively. The black filled square symbols represent the values of $D_0$.

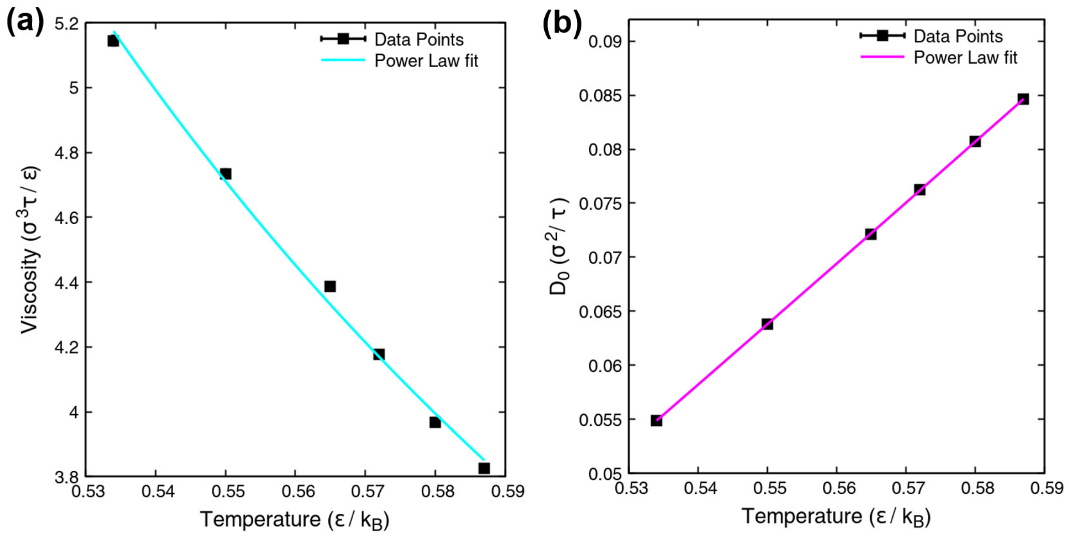


Figure S7: (a) Power law fit to the shear viscosities, for the LJ system. (b) Power law fit to the diffusion coefficients at zero shear, $D_0$, for the LJ system.

## References

(S1) Plimpton, S. Fast Parallel Algorithms for Short-Range Molecular Dynamics. *Journal of Computational Physics* **1995**, *117*, 1–19.

(S2) Evans, D. J.; Morriss, G. P. Nonlinear-response theory for steady planar Couette flow. *Physical Review A* **1984**, *30*, 1528–1530.

(S3) Lees, A. W.; Edwards, S. F. The computer study of transport processes under extreme conditions. *Journal of Physics C: Solid State Physics* **1972**, *5*, 1921–1928.

(S4) Daivis, P. J.; Todd, B. D. A simple, direct derivation and proof of the validity of the SLLOD equations of motion for generalized homogeneous flows. *The Journal of Chemical Physics* **2006**, *124*, 194103.

(S5) Shinoda, W.; Shiga, M.; Mikami, M. Rapid estimation of elastic constants by molecular dynamics simulation under constant stress. *Physical Review B* **2004**, *69*.

(S6) Abascal, J. L. F.; Vega, C. A general purpose model for the condensed phases of water: TIP4P/2005. *The Journal of Chemical Physics* **2005**, *123*, 234505.

(S7) Abascal, J. L. F.; Sanz, E.; Fernández, R. G.; Vega, C. A potential model for the study of ices and amorphous water: TIP4P/Ice. *The Journal of Chemical Physics* **2005**, *122*, 234511.

(S8) Molinero, V.; Moore, E. B. Water Modeled As an Intermediate Element between Carbon and Silicon†. *The Journal of Physical Chemistry B* **2009**, *113*, 4008–4016.

(S9) Broughton, J.; Gilmer, G. Surface free energy and stress of a Lennard-Jones crystal. *Acta Metallurgica* **1983**, *31*, 845–851.

(S10) R.W Hockney, J. W. E. *Computer simulation using particles*; crc Press, 1988.

(S11) Ryckaert, J.-P.; Ciccotti, G.; Berendsen, H. J. Numerical integration of the cartesian equations of motion of a system with constraints: molecular dynamics of n-alkanes. *Journal of Computational Physics* **1977**, *23*, 327–341.

(S12) Giorgino, T. Computing diffusion coefficients in macromolecular simulations: the Diffusion Coefficient Tool for VMD. *Journal of Open Source Software* **2019**, *4*, 1698.

(S13) Hess, B. Determining the shear viscosity of model liquids from molecular dynamics simulations. *The Journal of Chemical Physics* **2002**, *116*, 209.

(S14) Osipov, Y. A.; Zheleznyi, B.; Bondarenko, N. The shear viscosity of water supercooled to- 35 C. *Zh. Fiz. Khim* **1977**, *51*, 1264.

(S15) Dehaoui, A.; Issenmann, B.; Caupin, F. Viscosity of deeply supercooled water and its coupling to molecular diffusion. *Proceedings of the National Academy of Sciences* **2015**, *112*, 12020–12025.

(S16) Goswami, A.; Dalal, I. S.; Singh, J. K. Seeding method for ice nucleation under shear. *The Journal of Chemical Physics* **2020**, *153*, 094502.

(S17) Espinosa, J. R.; Sanz, E.; Valeriani, C.; Vega, C. Homogeneous ice nucleation evaluated for several water models. *The Journal of Chemical Physics* **2014**, *141*, 18C529.

(S18) Espinosa, J. R.; Vega, C.; Valeriani, C.; Sanz, E. Seeding approach to crystal nucleation. *The Journal of Chemical Physics* **2016**, *144*, 034501.

(S19) Quesnel, D. J.; Rimai, D. S.; DeMejo, L. P. Elastic compliances and stiffnesses of the fcc Lennard-Jones solid. *Physical Review B* **1993**, *48*, 6795–6807.

(S20) Feldman, C.; Klein, M. L. On the elastic constants of polycrystalline argon. *The Philosophical Magazine: A Journal of Theoretical Experimental and Applied Physics* **1968**, *17*, 135–140.

(S21) Gasser, U. Real-Space Imaging of Nucleation and Growth in Colloidal Crystallization. *Science* **2001**, *292*, 258–262.

(S22) Mura, F.; Zaccone, A. Effects of shear flow on phase nucleation and crystallization. *Physical Review E* **2016**, *93*.

(S23) Ohtori, N.; Uchiyama, H.; Ishii, Y. The Stokes-Einstein relation for simple fluids: From hard-sphere to Lennard-Jones via WCA potentials. *The Journal of Chemical Physics* **2018**, *149*, 214501.

(S24) Vega, C.; Abascal, J. L. F. Relation between the melting temperature and the temperature of maximum density for the most common models of water. *The Journal of Chemical Physics* **2005**, *123*, 144504.

(S25) Davidchack, R. L.; Laird, B. B. Direct calculation of the crystal–melt interfacial free energies for continuous potentials: Application to the Lennard-Jones system. *The Journal of Chemical Physics* **2003**, *118*, 7651.

(S26) Lee, S. H.; Kim, J. Transport properties of bulk water at 243–550 K: a Comparative

molecular dynamics simulation study using SPC/E, TIP4P, and TIP4P/2005 water models. *Molecular Physics* **2019**, *117*, 1926–1933.
